# Supplementary material for: Coulomb instabilities of 3D higher-order topological insulators
Source: arXiv:2103.02456 source file (2021-05-25)
Supplement: Supplementary file 1 [file Supplemental_Material.pdf]

# Supplemental Material for
# "Coulomb instabilities of 3D higher-order topological insulators"

Peng-Lu Zhao,[1,2] Xiao-Bin Qiang,[1,2] Hai-Zhou Lu,[1,2,*] and X. C. Xie[3,4,5]

[1] *Shenzhen Institute for Quantum Science and Engineering and Department of Physics, Southern University of Science and Technology (SUSTech), Shenzhen 518055, China*
[2] *Shenzhen Key Laboratory of Quantum Science and Engineering, Shenzhen 518055, China*
[3] *International Center for Quantum Materials, School of Physics, Peking University, Beijing 100871, China*
[4] *CAS Center for Excellence in Topological Quantum Computation, University of Chinese Academy of Sciences, Beijing 100190, China*
[5] *Beijing Academy of Quantum Information Sciences, West Building 3, No. 10, Xibeiwang East Road, Haidian District, Beijing 100193, China*

## CONTENTS

SI. Model and Symmetries S1

SII. Calculation of the Topological Invariant S2

SIII. Renormalization with only Coulomb interaction S3
A. Action with Coulomb interaction S3
B. One-loop corrections S5

SIV. Renormalization with disorder S8
A. Disorder action S8
B. One-Loop corrections S9
C. Renormalization group equations S12

SV. Influence of Coulomb interaction strength S14

SVI. Influence of disorder S14
A. Random mass S14
B. Random chemical potential S15

References S17

## SI. MODEL AND SYMMETRIES

The four-band model of a 3D second-order topological insulator is given by [1]

$$\mathcal{H}_0(\mathbf{k}) = \left[M + \sum_{i=x,y,z} t_i \cos(ak_i)\right] \tau_z\sigma_0 + \sum_{i=x,y,z} \Delta_i \sin(ak_i)\, \tau_x\sigma_i + \Delta_2 \left[\cos(ak_x) - \cos(ak_y)\right] \tau_y\sigma_0, \tag{S1}$$

where $a$ is the lattice constant, $M, t_{x,y,z}, \Delta_{x,y,z}, \Delta_2$ are the real hopping parameters, and $\sigma_i$ and $\tau_i$ are the three Pauli matrices for spin and orbital spaces, respectively. Hereafter, we take $t_x = t_y = t_\perp$, and $\Delta_x = \Delta_y = \Delta_\perp$.

* Corresponding author: luhz@sustech.edu.cn

The time-reversal operator is represented by $\mathcal{T} = \tau_0\sigma_y K$, where $K$ denotes the complex conjugate. The Hamiltonian Eq. (S1) under time-reversal transformation becomes

$$\begin{aligned}
&\mathcal{T}\mathcal{H}_0(\mathbf{k})\mathcal{T}^{-1} \\
&= \tau_0\sigma_y K\Big[\Big(M + \sum_{i=x,y,z} t_i\cos(ak_i)\Big)\tau_z\sigma_0 + \sum_{i=x,y,z}\Delta_i\sin(ak_i)\tau_x\sigma_i + \Delta_2\left[\cos(ak_x) - \cos(ak_y)\right]\tau_y\sigma_0\Big]K^{-1}\tau_0\sigma_y \\
&= \Big(M + \sum_{i=x,y,z} t_i\cos(ak_i)\Big)\tau_z\sigma_0 - \sum_{i=x,y,z}\Delta_i\sin(ak_i)\tau_x\sigma_i - \Delta_2\left[\cos(ak_x) - \cos(ak_y)\right]\tau_y\sigma_0 \\
&= \mathcal{H}_0(-\mathbf{k}) - 2\Delta_2\left[\cos(ak_x) - \cos(ak_y)\right]\tau_y\sigma_0. \qquad \text{(S2)}
\end{aligned}$$

As a result, $\mathcal{T}\mathcal{H}_0(\mathbf{k})\mathcal{T}^{-1} = \mathcal{H}_0(-\mathbf{k})$ if $\Delta_2 = 0$. The four-fold rotation operator along $z$-axes is represented by $R_{4z} = \tau_0 e^{-\mathrm{i}\frac{\pi}{4}\sigma_z}$. The Hamiltonian Eq. (S1) under this transformation becomes

$$\begin{aligned}
&R_{4z}\mathcal{H}_0(\mathbf{k})R_{4z}^{-1} \\
&= \tau_0 e^{-\mathrm{i}\frac{\pi}{4}\sigma_z}\Big[\Big(M + \sum_{i=x,y,z} t_i\cos(ak_i)\Big)\tau_z\sigma_0 + \sum_{i=x,y,z}\Delta_i\sin(k_i a)\,\tau_x\sigma_i + \Delta_2\left[\cos(ak_x) - \cos(ak_y)\right]\tau_y\sigma_0\Big]\tau_0 e^{\mathrm{i}\frac{\pi}{4}\sigma_z} \\
&= \Big[M + \sum_{i=x,y,z} t_i\cos(ak_i)\Big]\tau_z\sigma_0 + \tau_x\left[\Delta_\perp\left(\sin(ak_x)\sigma_y - \sin(ak_y)\sigma_x\right) + \Delta_z\sin(ak_z)\sigma_z\right] \\
&\quad +\Delta_2\left[\cos(ak_x) - \cos(ak_y)\right]\tau_y\sigma_0 \\
&= \mathcal{H}_0(-k_y, k_x, k_z) + 2\Delta_2\left[\cos(ak_x) - \cos(ak_y)\right]\tau_y\sigma_0. \qquad \text{(S3)}
\end{aligned}$$

As a result, $R_{4z}\mathcal{H}_0(\mathbf{k})R_{4z}^{-1} = \mathcal{H}_0(D_{R_{4z}}\mathbf{k})$ if $\Delta_2 = 0$, where $D_{\hat{R}_{4z}}(k_x, k_y, k_z) = (-k_y, k_x, k_z)$. The combination of the time-reversal and four-fold rotation gives rise to

$$\begin{aligned}
\left(R_{4z}\mathcal{T}\right)\mathcal{H}_0(\mathbf{k})\left(R_{4z}\mathcal{T}\right)^{-1} &= \left(R_{4z}\right)\left[\mathcal{H}_0(-\mathbf{k}) - 2\Delta_2\left[\cos(ak_x) - \cos(ak_y)\right]\tau_y\sigma_0\right]\left(R_{4z}\right)^{-1} \\
&= \mathcal{H}_0(k_y, -k_x, -k_z). \qquad \text{(S4)}
\end{aligned}$$

Therefore, the 3D second-order topological insulators break the time-reversal and four-fold rotation symmetries but respect their combination.

## SII. CALCULATION OF THE TOPOLOGICAL INVARIANT

The symmetry of $R_{4z}\mathcal{T}$ in the second-order topological insulators plays a role as time-reversal symmetry in topological insulators [1, 2]. For a 3D topological insulator, inversion symmetry plays a key role to simplify the calculation of the topological invariant [3]. Due to the breaking of inversion symmetry in the chiral second-order topological insulators, the role of inversion symmetry is replaced by the combination of time-reversal and inversion symmetry $\mathcal{I}\mathcal{T}$ with the representation $\mathcal{I} = \tau_z\sigma_0$. We first show the invariant of Hamiltonian Eq. (S1) under $\mathcal{I}\mathcal{T}$,

$$\begin{aligned}
(\mathcal{I}\mathcal{T})\mathcal{H}_0(\mathbf{k})(\mathcal{I}\mathcal{T})^{-1} &= \mathcal{I}\left[\mathcal{H}_0(-\mathbf{k}) - 2\Delta_2\left[\cos(ak_x) - \cos(ak_y)\right]\tau_y\sigma_0\right]\mathcal{I}^{-1} \\
&= \Big[M + \sum_{i=x,y,z} t_i\cos(ak_i)\Big]\tau_z\sigma_0 + \sum_{i=x,y,z}\Delta_i\sin(ak_i)\tau_x\sigma_i + \Delta_2\left[\cos(ak_x) - \cos(ak_y)\right]\tau_y\sigma_0 \\
&= \mathcal{H}_0(\mathbf{k}). \qquad \text{(S5)}
\end{aligned}$$

With this symmetry, we can take all the $R_{4z}\mathcal{T}$-invariant $\mathbf{k}$ points in the Brillouin zone to identify the topological invariant as [1, 3]

$$(-1)^\nu = \prod_i \prod_{n=1}^{N/2} \xi_n\left(\Gamma_i\right), \qquad \text{(S6)}$$

where $\xi_n\left(\Gamma_i\right) = \pm 1$ are the eigenvalues of $\mathcal{I}$ for the $n$-th occupied energy band at $\Gamma_i \in \{(0,0,0), (\pi,\pi,0), (0,0,\pi), (\pi,\pi,\pi)\}$, which account for all the $R_{4z}\mathcal{T}$-invariant $\mathbf{k}$ points. To calculate the topological invariant, we rewrite Eq. (S1) as

$$\mathcal{H}_0(\mathbf{k}) = d_0\left(\mathbf{k}\right)\gamma_0 + d_i\left(\mathbf{k}\right)\gamma_i + d_5\left(\mathbf{k}\right)\gamma_5 + d_{\mathcal{I}}\left(\mathbf{k}\right)\mathcal{I}_{4\times4}, \qquad \text{(S7)}$$

where $d_{\mathcal{I}}\left(\mathbf{k}\right) = 0$, and the particular forms of $d_{i=0,1,2,3,5}\left(\mathbf{k}\right)$ are given in Eq. (S1) by identifying $\gamma_0 = \tau_z\sigma_0, \gamma_{i=1,2,3} = \tau_x\sigma_{i=x,y,z}$, and $\gamma_5 = \tau_y\sigma_0$. According to Eq. (S3), we have

$$\begin{aligned}
&(R_{4z}\mathcal{T})\gamma_0(R_{4z}\mathcal{T})^{-1} = \gamma_0,\ (R_{4z}\mathcal{T})\gamma_1(R_{4z}\mathcal{T})^{-1} = -\gamma_2, \\
&(R_{4z}\mathcal{T})\gamma_2(R_{4z}\mathcal{T})^{-1} = \gamma_1,\ (R_{4z}\mathcal{T})\gamma_{3,5}(R_{4z}\mathcal{T})^{-1} = -\gamma_{3,5}. \qquad \text{(S8)}
\end{aligned}$$

At the $R_{4z}\mathcal{T}$-invariant $\mathbf{k}$ points, Eq. (S7) can be written as

$$\mathcal{H}_0(\Gamma_i) = d_0\left(\Gamma_i\right)\gamma_0 + d_1\left(\Gamma_i\right)\gamma_1 + d_2\left(\Gamma_i\right)\gamma_2 + d_{\mathcal{I}}(\Gamma_i)\mathcal{I}_{4\times 4}, \quad \left(d_{\mathcal{I}}(\Gamma_i) = 0\right), \tag{S9}$$

In addition, $d_1\left(\Gamma_i\right) = d_2\left(\Gamma_i\right) = 0$ for

$$\Gamma_i \in \{(0,0,0),(0,0,\pi),(\pi,\pi,0),(\pi,\pi,\pi)\}, \tag{S10}$$

we therefore obtain

$$\xi_{n=\text{valence}}\left(\Gamma_i\right) = -\text{sgn}(d_0\left(\Gamma_i\right)). \tag{S11}$$

As a consequence

$$(-1)^\nu = \prod_i \text{sgn}(d_0\left(\Gamma_i\right)) = \text{sgn}[(M+2t_\perp+t_z)(M-2t_\perp-t_z)(M+2t_\perp-t_z)(M-2t_\perp+t_z)]. \tag{S12}$$

Therefore, for $|2t_\perp - t_z| < |M| < |2t_\perp + t_z|$, $(-1)^\nu = -1$, which represents a second-order topological insulator and for $|M| > |2t_\perp + t_z|$ or $|M| < |2t_\perp - t_z|$, $(-1)^\nu = 1$, which stands for a normal insulator. We remind that despite the existences of the topological insulator and higher-order topological insulator share the same parameter constraint between $M$ and $t_i$, the appearance of the higher-order topological insulators additionally requires $d_5\left(\mathbf{k}\right) \neq -d_5\left(-\mathbf{k}\right)$ and $d_5\left(D_{\hat{R}_{4z}\hat{\mathcal{T}}}\mathbf{k}\right) = -d_5\left(\mathbf{k}\right)$.

## SIII. RENORMALIZATION WITH ONLY COULOMB INTERACTION

### A. Action with Coulomb interaction

For the model of Eq. (S1), the effective Hamiltonian density near the $\Gamma$ point reads

$$\begin{aligned}\mathcal{H}_0^{\text{e}}(\mathbf{k}) &= \left[M + 2t_\perp + t_z - \frac{t_\perp a^2}{2}\left(k_x^2 + k_y^2\right) + \frac{t_z a^2}{2}k_z^2\right]\tau_z\sigma_0 - \frac{\Delta_2 a^2}{2}\left(k_x^2 - k_y^2\right)\tau_y\sigma_0 \\ &\quad + a\tau_x\left[\Delta_\perp\left(k_x\sigma_x + k_y\sigma_y\right) + \Delta_z k_z\sigma_z\right] \\ &= \left[m - B_\perp\left(k_x^2 + k_y^2\right) - B_z k_z^2\right]\gamma_0 + \sum_i v_i k_i\gamma_i - D\left(k_x^2 - k_y^2\right)\gamma_5,\end{aligned} \tag{S13}$$

where $m = M + 2t_\perp + t_z, B_x = B_y = B_\perp = t_\perp a^2/2, B_z = t_z a^2/2, v_x = v_y = v = \Delta_\perp a, v_z = \Delta_z a$, and $D = \Delta_2 a^2/2$. The $\gamma$ matrices satisfy

$$\{\gamma_i, \gamma_j\} = 2\delta_{ij}, \quad \gamma_5 = -\gamma_0\gamma_1\gamma_2\gamma_3. \tag{S14}$$

The Bloch Hamiltonian is given by

$$H = \psi^\dagger\left[\left(m - B_i k_i^2\right)\gamma_0 + v_i k_i\gamma_i - D\left(k_x^2 - k_y^2\right)\gamma_5\right]\psi, \tag{S15}$$

where we have used a spinor basis $\psi^T = (c_{0,\uparrow}, c_{0,\downarrow}, c_{1,\uparrow}, c_{1,\downarrow})$, $c_{as}$ respectively correspond to the annihilation operators for electrons with spin projection $s$ in orbitals $\text{d}_{x^2-y^2}$ $(a=0)$ and $f_{z(x^2-y^2)}(a=1)$ [1]. Hereafter, the repeated $i$ sums automatically. The eigenvalues read

$$E_\pm^{\text{e}}(\mathbf{k}) = \pm E_{\mathbf{k}} = \pm\sqrt{\left[m - B_\perp\left(k_x^2 + k_y^2\right) - B_z k_z^2\right]^2 + v^2\left(k_x^2 + k_y^2\right) + v_z^2 k_z^2 + D^2\left(k_x^2 - k_y^2\right)^2}. \tag{S16}$$

The long-range Coulomb interaction between fermions is given by

$$H_C = \frac{1}{2}\int d^3\mathbf{r}d^3\mathbf{r}'\rho(\mathbf{r})\frac{e^2}{4\pi\epsilon\left|\mathbf{r}-\mathbf{r}'\right|}\rho(\mathbf{r}'), \tag{S17}$$

where $\rho(\mathbf{r}) = \psi^\dagger(\mathbf{r})\psi(\mathbf{r})$ is the normal-ordered electron density operator, $\epsilon$ is the dielectric constant and $-e$ is the electron charge. This kind of local density-density interaction does not explicitly break any lattice symmetry we discussed above. After performing a standard Hubbard-Stratonovich transformation, the action for the Coulomb interaction in the imaginary-time ($\tau = it$, $t$: time) formulation can be written as

$$S_C = \int d\tau d^3\mathbf{r}\left(ig\psi^\dagger\phi\psi\right) + \frac{1}{2}\int d\tau d^3\mathbf{r}\Big[\left(\partial_x\phi\right)^2 + \left(\partial_y\phi\right)^2 + \eta\left(\partial_z\phi\right)^2\Big], \tag{S18}$$

where $g = e/\sqrt{\epsilon}$ and $\phi$ is a bosonic field which is introduced through the Hubbard-Stratonovich transformation and the anisotropic variable $\eta$ is introduced due to the anisotropy of the dispersion generated by the nonzero $D$-term. The total action now reads

$$S = \int d\tau d^3\mathbf{r}\Big\{\psi^\dagger \left[(\partial_\tau + ig\phi) I + \left(m + B_i\partial_i^2\right)\gamma_0 - iv_i\gamma_i\partial_i + D\left(\partial_x^2 - \partial_y^2\right)\gamma_5\right]\psi + \frac{1}{2}\eta_i\left(\partial_i\phi\right)^2\Big\}, \tag{S19}$$

where $(\eta_x, \eta_y, \eta_z) = (1, 1, \eta)$ are used for short.

We explicitly show that the Coulomb part of the action preserves the symmetries $R_{4z}\mathcal{T}$ and $I\mathcal{T}$.

$$\begin{aligned}
&R_{4z}\mathcal{T}\int d\tau d^3\mathbf{r}\left\{ig\psi^\dagger\phi\psi + \frac{1}{2}\left[(\partial_x\phi)^2 + (\partial_y\phi)^2 + \eta\left(\partial_z\phi\right)^2\right]\right\}\mathcal{T}^{-1}\left(R_{4z}\right)^{-1}\\
&= R_{4z}\int d\tau d^3\mathbf{r}\left\{-ig\psi^\dagger(-i\tau_0\sigma_y)(i\tau_0\sigma_y)\psi(-\phi) + \frac{1}{2}\left[(-\partial_x\phi)^2 + (-\partial_y\phi)^2 + \eta\left(-\partial_z\phi\right)^2\right]\right\}\left(R_{4z}\right)^{-1}\\
&= \int d\tau d^3\mathbf{r}\left\{ig\psi^\dagger\psi\phi + \frac{1}{2}\left[(\partial_x\phi)^2 + (\partial_y\phi)^2 + \eta\left(\partial_z\phi\right)^2\right]\right\},
\end{aligned} \tag{S20}$$

where we have used the transformations directly

$$\mathcal{T}\psi\mathcal{T}^{-1} = \left(c_{0,\downarrow}, -c_{0,\uparrow}, c_{1,\downarrow}, -c_{1,\uparrow}\right)^{\mathrm{T}} = i\tau_0\sigma_y\psi, \quad \mathcal{T}\phi\mathcal{T}^{-1} = -\phi. \tag{S21}$$

For the inversion transformation,

$$\mathcal{I}\psi(\mathbf{r})\mathcal{I}^{-1} = \tau_z\sigma_0\psi(-\mathbf{r}), \quad \mathcal{I}\phi(\mathbf{r})\mathcal{I}^{-1} = \phi(-\mathbf{r}). \tag{S22}$$

Therefore,

$$\begin{aligned}
&\mathcal{I}\mathcal{T}\int d\tau d^3\mathbf{r}\left\{ig\psi^\dagger\phi\psi + \frac{1}{2}\left[(\partial_x\phi)^2 + (\partial_y\phi)^2 + \eta\left(\partial_z\phi\right)^2\right]\right\}\mathcal{T}^{-1}\mathcal{I}^{-1}\\
&= \mathcal{I}\int d\tau d^3\mathbf{r}\left\{-ig\psi^\dagger(-\mathbf{r})(-i\tau_0\sigma_y)(i\tau_0\sigma_y)\psi(-\mathbf{r})(-\phi(-\mathbf{r})) + \frac{1}{2}\left[(-\partial_x\phi)^2 + (-\partial_y\phi)^2 + \eta\left(-\partial_z\phi\right)^2\right]\right\}\mathcal{I}^{-1}\\
&= \int d\tau d^3\mathbf{r}\left\{ig\psi^\dagger\psi\phi + \frac{1}{2}\left[(\partial_x\phi)^2 + (\partial_y\phi)^2 + \eta\left(\partial_z\phi\right)^2\right]\right\}.
\end{aligned} \tag{S23}$$

Therefore, the topological invariants defined by Eq. (S6) still hold in the presence of the weak Coulomb interaction.

Define $\bar{\psi} = \psi^\dagger\gamma_0$, the total action is reshaped as

$$\mathcal{S} = \int d\tau d^3\mathbf{r}\Big\{\bar{\psi}\left[(\partial_\tau + ig\phi)\gamma_0 + \left(m + B_i\partial_i^2\right)I + v_i\tilde{\gamma}_i\partial_i - iD\left(\partial_x^2 - \partial_y^2\right)\tilde{\gamma}_5\right]\psi + \frac{1}{2}\eta_i\left(\partial_i\phi\right)^2\Big\}, \tag{S24}$$

where $\tilde{\gamma}_i = \tau_y\sigma_i$, $\tilde{\gamma}_5 = \tau_x\sigma_0$, and we make the replacements: $\tilde{\gamma}_i \to \gamma_i, \tilde{\gamma}_5 \to \gamma_5$ in the main text. Although we change the specific expressions for the $\gamma$ matrices, the $\gamma$-algebra Eq. (S14) is unchanged. According to Eq. (S24), the free propagator of fermions reads

$$\left\langle\mathcal{T}_\tau\left\{\psi\left(X_1\right)\bar{\psi}\left(X_2\right)\right\}\right\rangle = \int_{k_0,\mathbf{k}} e^{ik_0(\tau_1-\tau_2)+i\mathbf{k}\cdot(\mathbf{r}_1-\mathbf{r}_2)}G_0\left(k_0,\mathbf{k}\right), \tag{S25}$$

with

$$G_0\left(k_0,\mathbf{k}\right) = \frac{1}{i\left[k_0\gamma_0 + v_i\gamma_i k_i + D\left(k_x^2 - k_y^2\right)\gamma_5\right] + m - B_i k_i^2}. \tag{S26}$$

The free propagator of the bosonic field:

$$\left\langle\mathcal{T}_\tau\left\{\phi\left(X_1\right)\phi\left(X_2\right)\right\}\right\rangle = \int_{\omega,\mathbf{k}} e^{ik_0(\tau_1-\tau_2)+i\mathbf{k}\cdot(\mathbf{r}_1-\mathbf{r}_2)}D_0\left(k_0,\mathbf{k}\right), \tag{S27}$$

with

$$D_0\left(k_0,\mathbf{k}\right) = \frac{1}{k_x^2 + k_y^2 + \eta k_z^2}. \tag{S28}$$

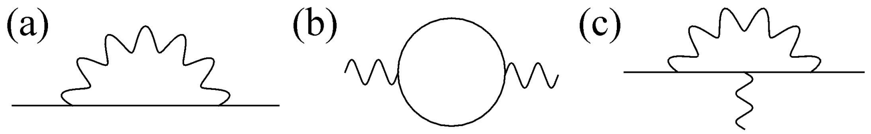


FIG. S1. The Feynman diagrams for the one-loop corrections to the fermion self-energy (a), scalar potential self-energy (b), and vertex (c). The solid and wavy lines stand for the fermion and scalar boson, respectively.

### B. One-loop corrections

**Electron self-energy.** We first calculate the one-loop fermionic self-energy shown in Fig. S1(a), which gives rise to the renormalization of $v_i$, $B_i$, $D$, and $m$. At one-loop order, $\Sigma(k)$ can be written as

$$\begin{aligned}\Sigma\left(k_0,\mathbf{k}\right) &= -g^2\int_{-\infty}^{\infty}\frac{dq_0}{2\pi}\int'\frac{d^3q}{(2\pi)^3}\gamma_0 G_0(q)\gamma_0 D_0(k-q)\\ &= -g^2\int'\frac{d^3q}{(2\pi)^3}\int_{-\infty}^{\infty}\frac{dq_0}{2\pi}\frac{m-B_iq_i^2-i\left[q_0\gamma_0-v_i\gamma_iq_i-D\left(q_x^2-q_y^2\right)\gamma_5\right]}{\left(q_0^2+E_{\mathbf{q}}^2\right)\left[\left(k_x-q_x\right)^2+\left(k_y-q_y\right)^2+\eta\left(k_z-q_z\right)^2\right]},\end{aligned} \tag{S29}$$

where $E_{\mathbf{q}}$ is defined in Eq. (S16) and $\int'\frac{d^3q}{(2\pi)^3}$ indicates the integral over the momentum shell. Due to the space anisotropy, we employ a momentum shell as $\Lambda e^{-\ell}<\sqrt{q_\perp^2+\eta q_z^2}<\Lambda$. In the following, the momentum integral is performed by

$$\int' d^3q = \int'\frac{d^3q'}{\sqrt{\eta}} = \int_{\Lambda e^{-\ell}}^{\Lambda}\frac{q'^2dq'}{\sqrt{\eta}}\int d\Omega, \tag{S30}$$

where $\mathbf{q}'=\left(q_x,q_y,\sqrt{\eta}q_z\right)$, $\int d\Omega=\int_0^\pi\sin\varphi d\varphi\int_0^{2\pi}d\theta$, and the spherical coordinates is used, in particular

$$q_x=q'\sin\varphi\cos\theta,\quad q_y=q'\sin\varphi\sin\theta,\quad q_z'=q'\cos\varphi. \tag{S31}$$

To calculate Eq. (S29), we expand $\Sigma\left(k_0,\mathbf{k}\right)$ in powers of $k_i$ up to quadratic order, and obtain

$$\Sigma\left(k_0,\mathbf{k}\right)=\Sigma_0+\Sigma_{1\perp}iv\left(\gamma_xk_x+\gamma_yk_y\right)+\Sigma_{1z}iv_z\gamma_zk_z+\Sigma_{2\perp}\left(k_x^2+k_y^2\right)+\Sigma_{2z}k_z^2+\Sigma_{2D}iD\gamma_5\left(k_x^2-k_y^2\right). \tag{S32}$$

$\Sigma_0$ is given by

$$\begin{aligned}\Sigma_0 &= -\frac{g^2}{2}\int'\frac{d^3q}{(2\pi)^3}\frac{\left(m-B_iq_i^2\right)+iD\left(q_x^2-q_y^2\right)\gamma_5}{\left(q_x^2+q_y^2+\eta q_z^2\right)\sqrt{\left(m-B_iq_i^2\right)^2+v_i^2q_i^2+D^2\left(q_x^2-q_y^2\right)^2}}\\ &= \frac{-g^2\ell}{4\pi^2v\sqrt{\eta}}\frac{1}{4\pi}\int_0^\pi\sin\varphi d\varphi\int_0^{2\pi}d\theta\\ &\quad\times\frac{v\Lambda\left[mv^{-1}\Lambda^{-1}-\left(B_\perp\sin^2\varphi+B_z\eta^{-1}\cos^2\varphi\right)\Lambda v^{-1}\right]+iD\gamma_5\Lambda^2\sin^2\varphi\cos2\theta}{\sqrt{\left[mv^{-1}\Lambda^{-1}-\left(B_\perp\sin^2\varphi+B_z\eta^{-1}\cos^2\varphi\right)\Lambda v^{-1}\right]^2+\sin^2\varphi+\gamma^2\cos^2\varphi+\left(D\Lambda v^{-1}\right)^2\sin^4\varphi\cos^22\theta}},\end{aligned} \tag{S33}$$

where $\gamma=v_z/(v\sqrt{\eta})$. By identifying the following dimensionless effective parameters:

$$B_i\Lambda v^{-1}\eta_i^{-1}\to B_i,\quad D\Lambda v^{-1}\to D,\quad mv^{-1}\Lambda^{-1}\to m,\quad g^2/(4\pi^2v\sqrt{\eta})\to\alpha, \tag{S34}$$

Eq. (S33) can be rewritten by the redefined parameters as

$$\Sigma_0=-\alpha\ell v\Lambda\left[m\left(\mathcal{F}_0^\perp+\mathcal{F}_0^z\right)-B_\perp\mathcal{F}_0^\perp-B_z\mathcal{F}_0^z\right], \tag{S35}$$

where

$$\mathcal{F}_0^\perp\left(m,B_i,D,\gamma\right)=\int\frac{d\Omega}{4\pi}\frac{\sin^2\varphi}{\sqrt{\left[m-\left(B_\perp\sin^2\varphi+B_z\cos^2\varphi\right)\right]^2+\sin^2\varphi+\gamma^2\cos^2\varphi+D^2\sin^4\varphi\cos^22\theta}}, \tag{S36}$$

$$\mathcal{F}_0^z\left(m,B_i,D,\gamma\right)=\int\frac{d\Omega}{4\pi}\frac{\cos^2\varphi}{\sqrt{\left[m-\left(B_\perp\sin^2\varphi+B_z\cos^2\varphi\right)\right]^2+\sin^2\varphi+\gamma^2\cos^2\varphi+D^2\sin^4\varphi\cos^22\theta}}. \tag{S37}$$

$$\Sigma_{1\perp} = -\frac{g^2}{2}\int' \frac{d^3q}{(2\pi)^3}\frac{q_\perp^2}{\left(q_x^2+q_y^2+\eta q_z^2\right)^2\sqrt{\left(m-B_iq_i^2\right)^2+v_i^2q_i^2+D^2\left(q_x^2-q_y^2\right)^2}}$$
$$= -\alpha\ell\mathcal{F}_0^{\perp}\left(m,B_i,D,\gamma\right), \tag{S38}$$

$$\Sigma_{1z} = -\frac{g^2}{2}\int' \frac{d^3q}{(2\pi)^3}\frac{2\eta q_z^2}{\left(q_x^2+q_y^2+\eta q_z^2\right)^2\sqrt{\left(m-B_iq_i^2\right)^2+v_i^2q_i^2+D^2\left(q_x^2-q_y^2\right)^2}}$$
$$= -2\alpha\ell\mathcal{F}_0^{z}\left(m,B_i,D,\gamma\right), \tag{S39}$$

$$\Sigma_{2\perp} = -\frac{g^2}{2}\int' \frac{d^3q}{(2\pi)^3}\frac{\left(q_x^2+q_y^2-\eta q_z^2\right)\left(m-B_iq_i^2\right)}{\left(q_x^2+q_y^2+\eta q_z^2\right)^3\sqrt{\left(m-B_iq_i^2\right)^2+v_i^2q_i^2+D^2\left(q_x^2-q_y^2\right)^2}}$$
$$= -\alpha\ell v\Lambda^{-1}\left[m\left(\mathcal{F}_1^{\perp}+\mathcal{F}_1^{z}\right)-B_\perp\mathcal{F}_1^{\perp}-B_z\mathcal{F}_1^{z}\right], \tag{S40}$$

where

$$\mathcal{F}_1^{\perp}\left(m,B_i,D,\gamma\right) = \int\frac{d\Omega}{4\pi}\frac{-\cos 2\varphi\sin^2\varphi}{\sqrt{\left[m-\left(B_\perp\sin^2\varphi+B_z\cos^2\varphi\right)\right]^2+\sin^2\varphi+\gamma^2\cos^2\varphi+D^2\sin^4\varphi\cos^2 2\theta}}, \tag{S41}$$

$$\mathcal{F}_1^{z}\left(m,B_i,D,\gamma\right) = \int\frac{d\Omega}{4\pi}\frac{-\cos 2\varphi\cos^2\varphi}{\sqrt{\left[m-\left(B_\perp\sin^2\varphi+B_z\cos^2\varphi\right)\right]^2+\sin^2\varphi+\gamma^2\cos^2\varphi+D^2\sin^4\varphi\cos^2 2\theta}}. \tag{S42}$$

The defined $\mathcal{F}_0^{\perp},\mathcal{F}_0^{z},\mathcal{F}_1^{\perp},\mathcal{F}_1^{z}$ are not fully independent. Instead, they satisfy

$$\mathcal{F}_0^{\perp} = \mathcal{F}_0^{z}+\mathcal{F}_1^{\perp}+\mathcal{F}_1^{z}. \tag{S43}$$

$$\Sigma_{2z} = -\frac{g^2}{2}\int' \frac{d^3q}{(2\pi)^3}\frac{\eta\left(3\eta q_z^2-q_x^2-q_y^2\right)\left(m-B_iq_i^2\right)}{\left(q_x^2+q_y^2+\eta q_z^2\right)^3\sqrt{\left(m-B_iq_i^2\right)^2+v_i^2q_i^2+D^2\left(q_x^2-q_y^2\right)^2}}$$
$$= -\alpha\ell v\Lambda^{-1}\eta\left\{m\left[\mathcal{F}_0^{\perp}+\mathcal{F}_0^{z}-2\left(\mathcal{F}_1^{\perp}+\mathcal{F}_1^{z}\right)\right]-B_\perp\left(\mathcal{F}_0^{\perp}-2\mathcal{F}_1^{\perp}\right)-B_z\left(\mathcal{F}_0^{z}-2\mathcal{F}_1^{z}\right)\right\}, \tag{S44}$$

$$\Sigma_{2D} = -\frac{g^2}{2}\int' \frac{d^3q}{(2\pi)^3}\frac{2\left(q_y^2-q_x^2\right)^2}{\left(q_x^2+q_y^2+\eta q_z^2\right)^3\sqrt{\left(m-B_iq_i^2\right)^2+v_i^2q_i^2+D^2\left(q_x^2-q_y^2\right)^2}}$$
$$= -\alpha\mathcal{F}_1^{D}\left(m,B_i,D,\gamma\right)\ell, \tag{S45}$$

where we define

$$\mathcal{F}_1^{D}\left(m,B_i,D,\gamma\right) = \int\frac{d\Omega}{4\pi}\frac{2\sin^4\varphi\cos^2 2\theta}{\sqrt{\left[m-\left(B_\perp\sin^2\varphi+B_z\cos^2\varphi\right)\right]^2+\sin^2\varphi+\gamma^2\cos^2\varphi+D^2\sin^4\varphi\cos^2 2\theta}}. \tag{S46}$$

In summary, the fermion self-energy correction reads

$$\begin{aligned}\Sigma\left(k_0,\mathbf{k}\right) = &-\alpha\ell v\Lambda\left[m\left(\mathcal{F}_0^{\perp}+\mathcal{F}_0^{z}\right)-B_\perp\mathcal{F}_0^{\perp}-B_z\mathcal{F}_0^{z}\right]-\alpha\ell\left[iv\mathcal{F}_0^{\perp}\left(\gamma_xk_x+\gamma_yk_y\right)+2iv_z\mathcal{F}_0^{z}\left(\gamma_zk_z\right)\right]\\ &-\alpha v\Lambda^{-1}\ell\Big\{\left[m\left(\mathcal{F}_1^{\perp}+\mathcal{F}_1^{z}\right)-B_\perp\mathcal{F}_1^{\perp}-B_z\mathcal{F}_1^{z}\right]\left(k_x^2+k_y^2\right)+\eta\Big[m\left[\mathcal{F}_0^{\perp}+\mathcal{F}_0^{z}-2\left(\mathcal{F}_1^{\perp}+\mathcal{F}_1^{z}\right)\right]\\ &-B_\perp\left(\mathcal{F}_0^{\perp}-2\mathcal{F}_1^{\perp}\right)-B_z\left(\mathcal{F}_0^{z}-2\mathcal{F}_1^{z}\right)\Big]k_z^2\Big\}-\alpha\mathcal{F}_1^{D}v\Lambda^{-1}\ell iD\gamma_5\left(k_x^2-k_y^2\right).\end{aligned} \tag{S47}$$

This correction adds a term in the renormalized action according to

$$\bar{\psi}\left[G_0^{-1}\left(k\right)-\Sigma\left(k_0,\mathbf{k}\right)\right]\psi. \tag{S48}$$

**Scalar potential self-energy:** We now calculate the one-loop boson self-energy $\Pi(k)$ as shown in Fig. S1(b), which is given by

$$\begin{aligned}\Pi(k) &= g^2\int_{-\infty}^{\infty}\frac{dq_0}{2\pi}\int'\frac{d^3q}{(2\pi)^3}\,\mathrm{Tr}\left[\gamma_0 G_0(q)\gamma_0 G_0(k+q)\right]\\&= -4g^2\int_{-\infty}^{\infty}\frac{dq_0}{2\pi}\int'\frac{d^3q}{(2\pi)^3}\frac{1}{\left(q_0^2+E_{\mathbf{q}}^2\right)\left[\left(q_0+k_0\right)^2+E_{\mathbf{q+k}}^2\right]}\Big\{q_0\left(q_0+k_0\right)-v_i^2q_i\left(q_i+k_i\right)\\&\quad-\left(m-B_iq_i^2\right)\left[m-B_i\left(k_i+q_i\right)^2\right]-D^2\left(q_x^2-q_y^2\right)\left[\left(q_x+k_x\right)^2-\left(q_y+k_y\right)^2\right]\Big\},\end{aligned}\tag{S49}$$

To calculate Eq. (S49), we expand $\Pi(k)$ in powers of $k_i$ up to quadratic order, for powers of $k_0$, we have

$$\Pi_0(k)\approx -4g^2\int'\frac{d^3q}{(2\pi)^3}\int_{-\infty}^{\infty}\frac{dq_0}{2\pi}\left[\frac{q_0^2-E_{\mathbf{q}}^2}{\left(q_0^2+E_{\mathbf{q}}^2\right)^2}+\frac{\left(q_0^4-6q_0^2E_{\mathbf{q}}^2+E_{\mathbf{q}}^4\right)k_0^2}{\left(q_0^2+E_{\mathbf{q}}^2\right)^4}\right]=0.\tag{S50}$$

For powers of $\mathbf{k}$, we first finish the integral of $q_0$ and then make the series expansion, and obtain

$$\begin{aligned}\Pi(k)&\approx -4g^2\int'\frac{d^3q}{(2\pi)^3}\left\{\frac{E_{\mathbf{q}}^2\left[4q_x^2\left(B_\perp^2+D^2\right)+v^2\right]-q_x^2\left[2B_\perp B_iq_i^2-2B_\perp m+2D^2\left(q_x^2-q_y^2\right)+v^2\right]^2}{8E_{\mathbf{q}}^5}k_x^2\right.\\&\quad+\frac{E_{\mathbf{q}}^2\left[4q_y^2\left(B_\perp^2+D^2\right)+v^2\right]-q_y^2\left[2B_\perp B_iq_i^2-2B_\perp m+2D^2\left(q_y^2-q_x^2\right)+v^2\right]^2}{8E_{\mathbf{q}}^5}k_y^2\\&\quad\left.+\frac{E_{\mathbf{q}}^2\left(4q_z^2B_z^2+v_z^2\right)-q_z^2\left(2B_zB_iq_i^2-2B_zm+v_z^2\right)^2}{8E_{\mathbf{q}}^5}k_z^2\right\}\\&=\Pi_xk_x^2+\Pi_yk_y^2+\Pi_zk_z^2.\end{aligned}\tag{S51}$$

Therefore,

$$\begin{aligned}\Pi_x&=-4g^2\int'\frac{d^3q}{(2\pi)^3}\frac{E_{\mathbf{q}}^2\left[4q_x^2\left(B_\perp^2+D^2\right)+v^2\right]-q_x^2\left[2B_\perp B_iq_i^2-2B_\perp m+2D^2\left(q_x^2-q_y^2\right)+v^2\right]^2}{8E_{\mathbf{q}}^5}\\&=-\alpha\ell\mathcal{F}_2^\perp\left(m,B_i,D,\gamma\right),\end{aligned}\tag{S52}$$

and $\mathcal{F}_2\left(m,B_i,D,\gamma\right)$ is given by

$$\begin{aligned}\mathcal{F}_2^\perp&=\frac{1}{4\pi}\int_0^\pi\sin\varphi d\varphi\int_0^{2\pi}d\theta\left\{\frac{4\sin^2\varphi\cos^2\theta\left(B_\perp^2+D^2\right)+1}{\left[\left[m-\left(B_\perp\sin^2\varphi+B_z\cos^2\varphi\right)\right]^2+\sin^2\varphi+\gamma^2\cos^2\varphi+D^2\sin^4\varphi\cos^2 2\theta\right]^{3/2}}\right.\\&\quad\left.-\frac{\sin^2\varphi\cos^2\theta\left[2B_\perp\left(B_\perp\sin^2\varphi+B_z\cos^2\varphi\right)-2B_\perp m+2D^2\sin^2\varphi\cos 2\theta+1\right]^2}{\left[\left[m-\left(B_\perp\sin^2\varphi+B_z\cos^2\varphi\right)\right]^2+\sin^2\varphi+\gamma^2\cos^2\varphi+D^2\sin^4\varphi\cos^2 2\theta\right]^{5/2}}\right\}.\end{aligned}\tag{S53}$$

By exchanging $q_x$ and $q_y$, we have $\Pi_x\leftrightarrow\Pi_y$, therefore,

$$\Pi_y=\Pi_x=-\alpha\ell\mathcal{F}_2^\perp\left(m,B_i,D,\gamma\right).\tag{S54}$$

For $\Pi_z$, we obtain

$$\begin{aligned}\Pi_z&=-4g^2\int'\frac{d^3q}{(2\pi)^3}\frac{E_{\mathbf{q}}^2\left(4q_z^2B_z^2+v_z^2\right)-q_z^2\left(2B_zB_iq_i^2-2B_zm+v_z^2\right)^2}{8E_{\mathbf{q}}^5}\\&=\frac{-\alpha\ell}{4\pi}\int d\Omega\left\{\frac{4B_z^2\cos^2\varphi+\gamma^2}{\left[\left(m-B\right)^2+1+D^2\sin^4\varphi\cos^2 2\theta\right]^{3/2}}-\frac{\cos^2\varphi\left(2B_z^2-2B_zm+\gamma^2\right)^2}{\left[\left(m-B\right)^2+1+D^2\sin^4\varphi\cos^2 2\theta\right]^{5/2}}\right\}\\&=-\alpha\eta\mathcal{F}_2^z\left(m,B_i,D,\gamma\right)\ell,\end{aligned}\tag{S55}$$

where $\mathcal{F}_2^z\left(m, B_i, D, \gamma\right)$ takes the form

$$\mathcal{F}_2^z = \frac{1}{4\pi}\int_0^{\pi}\sin\varphi d\varphi\int_0^{2\pi}d\theta\left\{\frac{4B_z^2\cos^2\varphi+\gamma^2}{\left[\left[m-\left(B_\perp\sin^2\varphi+B_z\cos^2\varphi\right)\right]^2+\sin^2\varphi+\gamma^2\cos^2\varphi+D^2\sin^4\varphi\cos^2 2\theta\right]^{3/2}}\right.$$
$$\left.-\frac{\cos^2\varphi\left[2B_z\left(B_\perp\sin^2\varphi+B_z\cos^2\varphi\right)-2B_z m+\gamma^2\right]^2}{\left[\left[m-\left(B_\perp\sin^2\varphi+B_z\cos^2\varphi\right)\right]^2+\sin^2\varphi+\gamma^2\cos^2\varphi+D^2\sin^4\varphi\cos^2 2\theta\right]^{5/2}}\right\}. \tag{S56}$$

In summary, the boson self-energy takes the form

$$\Pi(k) = -\alpha\mathcal{F}_2^\perp\left(m, B_i, D, \gamma\right)\ell\left(k_x^2+k_y^2\right)-\alpha\mathcal{F}_2^z\left(m, B_i, D, \gamma\right)\ell\eta k_z^2. \tag{S57}$$

This correction contributes a term in the renormalized action by

$$\phi\left[D_0^{-1}(k)-\frac{\Pi(k)}{2}\right]\phi. \tag{S58}$$

**Vertex correction.** For the vertex correction we find at vanishing external momentum and frequency

$$\begin{aligned}\delta g_1 &= -g^2\int_{-\infty}^{\infty}\frac{dq_0}{2\pi}\int'\frac{d^3q}{(2\pi)^3}G_0(q)\gamma_0 G_0(q)\gamma_0 D(q)\\ &= -g^2\int'\frac{d^3q}{(2\pi)^3}\int_{-\infty}^{\infty}\frac{dq_0}{2\pi}\frac{E_{\mathbf{q}}^2-q_0^2}{\left(q_0^2+E_{\mathbf{q}}^2\right)^2\left(q_x^2+q_y^2+\eta q_z^2\right)}\\ &= 0.\end{aligned} \tag{S59}$$

This result is also a consequence of the $U(1)$ gauge symmetry. To be concrete, we check that the action is invariant under this gauge transformation

$$\psi\to e^{-i\chi(\tau)}\psi, \phi\to\phi+\frac{1}{g}\partial_\tau\chi. \tag{S60}$$

Counting the loop corrections, the related invariant action now is

$$S\to\int d\tau d^3\mathbf{r}\bar{\psi}\left\{\left[\left(1+\Sigma_\omega\right)\partial_\tau+ig\left(1+\delta g_1\right)\phi\right]\gamma_0\right\}\psi. \tag{S61}$$

Under the gauge transformation the action becomes

$$S\to\int d\tau d^3\mathbf{r}\bar{\psi}\left\{\left[\left(1+\Sigma_\omega\right)\partial_\tau+ig\left(1+\delta g_1\right)\phi+i\partial_\tau\chi\left(\tau\right)\left(\delta g_1-\Sigma_\omega\right)\right]\gamma_0\right\}\psi. \tag{S62}$$

To be gauge invariant, we must have

$$\delta g_1 = \Sigma_\omega. \tag{S63}$$

Because the propagator for the boson is independent on zero-momentum, the self-energy correction does not contain a zero-momentum term, which means $\Sigma_\omega = 0$, and this result holds for any loops. As a result,

$$\delta g_1 = \Sigma_\omega = 0. \tag{S64}$$

## SIV. RENORMALIZATION WITH DISORDER

### A. Disorder action

The fermion-disorder coupling is generally described by [4–7],

$$S_{\text{dis}} = \int d^3\mathbf{r}d\tau\psi^\dagger\left(\sum_j A_j(\mathbf{r})M_j\right)\psi, \tag{S65}$$

TABLE S1. Types of disorder represented by various fermionic bilinears and their symmetries under $R_{4z}\mathcal{T}$ and $\mathcal{IT}$. Here $\pm 1$ represents $\mathcal{O}\left(\psi^{\dagger}M\psi\right)\mathcal{O}^{-1}=\pm\left(\psi^{\dagger}M\psi\right)$, while $\bigotimes$ signifies $\mathcal{O}\left(\psi^{\dagger}M\psi\right)\mathcal{O}^{-1}\neq k\left(\psi^{\dagger}M\psi\right)$, where $\mathcal{O}$ stands for $R_{4z}\mathcal{T}$ or $\mathcal{IT}$, and $k$ is any complex number.

| Bilinears | $R_{4z}\mathcal{T}$ | $\mathcal{IT}$ | Disorder average |
|---|---|---|---|
| $\psi^{\dagger}\psi$ | $+1$ | $+1$ | $\langle A_0(\mathbf{r})A_0(\mathbf{r}')\rangle=\Delta_C\delta^3(\mathbf{r}-\mathbf{r}')$ |
| $\psi^{\dagger}\tau_0\sigma_{(x,y)}\psi$ | $\bigotimes$ | $-1$ | |
| $\psi^{\dagger}\tau_0\sigma_z\psi$ | $-1$ | $-1$ | |
| $\psi^{\dagger}\tau_x\sigma_0\psi$ | $+1$ | $-1$ | |
| $\psi^{\dagger}\tau_x\sigma_{(x,y)}\psi$ | $\bigotimes$ | $+1$ | |
| $\psi^{\dagger}\tau_x\sigma_z\psi$ | $-1$ | $+1$ | |
| $\psi^{\dagger}\tau_y\sigma_0\psi$ | $-1$ | $+1$ | |
| $\psi^{\dagger}\tau_y\sigma_{(x,y)}\psi$ | $\bigotimes$ | $-1$ | |
| $\psi^{\dagger}\tau_y\sigma_z\psi$ | $+1$ | $-1$ | |
| $\psi^{\dagger}\tau_z\sigma_0\psi$ | $+1$ | $+1$ | $\langle A_1(\mathbf{r})A_1(\mathbf{r}')\rangle=\Delta_M\delta^3(\mathbf{r}-\mathbf{r}')$ |
| $\psi^{\dagger}\tau_z\sigma_{(x,y)}\psi$ | $\bigotimes$ | $-1$ | |
| $\psi^{\dagger}\tau_z\sigma_z\psi$ | $-1$ | $-1$ | |

where the function $A_j(\mathbf{r})$ stands for the randomly distributed potential and $M_j$ is a $4\times 4$ Hermitian matrix. We assume $A_j(\mathbf{r})$ to be a quenched, Gaussian white noise potential characterized by the following identities

$$\langle A_j(\mathbf{r})\rangle=0,\qquad \langle A_j(\mathbf{r})A_l(\mathbf{r}')\rangle=\Delta_j\delta_{jl}\delta^3(\mathbf{r}-\mathbf{r}'). \tag{S66}$$

Here, the dimensionless variances $\Delta_i$ are introduced to characterize the strengths of random potentials. The disorder type is determined by $M_j$, which contains sixteen independent possibilities. By requiring that disorder should respect the symmetries protecting the topology, only two types of disorder need to consider. We have summarized various types of disorder and their symmetries under $R_{4z}\mathcal{T}$ and $\mathcal{IT}$ in Tab. S1. According to Tab. S1, we only consider disorder denoted by $M_0=I_{4\times 4}$ and $M_1=\gamma_0=\tau_z\sigma_0$, which represent the random chemical potential and random mass [4, 7], respectively.

The random potential $A_j(\mathbf{r})$ needs to be properly averaged. To do this, we assume that the spatial distribution of $A_j(\mathbf{r})$ is described by $P\left[A_j\right]=\exp\left[-\int d^3\mathbf{r}A_j^2(\mathbf{r})/(2\Delta_j)\right]$. By employing the most widely used replica method [8–10] to perform the disorder average, we obtain an effective replicated action in the Euclidean space

$$S_{\text{dis}}=-\frac{1}{2}\int d^3\mathbf{r}d\tau d\tau'\left[\Delta_M\left(\bar{\psi}_m\psi_m\right)_r\left(\bar{\psi}_n\psi_n\right)_{r'}+\Delta_C\left(\bar{\psi}_m\gamma_0\psi_m\right)_r\left(\bar{\psi}_n\gamma_0\psi_n\right)_{r'}\right]. \tag{S67}$$

Here, $r\equiv(\mathbf{r},\tau)$, $r'\equiv(\mathbf{r},\tau')$, $m$ and $n$ are the replica indices which are summed up automatically.

### B. One-Loop corrections

All the Feynman diagrams generated by disorder are shown in Fig. S2. Fig. S2(a) represents the disorder-induced self-energy correction, which is given by

$$\begin{aligned}\Sigma_{\text{dis}}^{(a)}(k_0)&=-\int\frac{d^3\mathbf{k}}{(2\pi)^3}\left[\Delta_M G_0(k_0,\mathbf{k})+\Delta_C\gamma_0 G_0(k_0,\mathbf{k})\gamma_0\right]\\&=-\frac{(\Delta_M+\Delta_C)\Lambda\ell}{2\pi^2v^2\sqrt{\eta}}\left\{-ik_0\gamma_0\left(\mathcal{G}_0^{\perp}+\mathcal{G}_0^{z}\right)+v\Lambda\left[m\left(\mathcal{G}_0^{\perp}+\mathcal{G}_0^{z}\right)-B_{\perp}\mathcal{G}_0^{\perp}-B_z\mathcal{G}_0^{z}\right]\right\},\end{aligned} \tag{S68}$$

where

$$\mathcal{G}_0^{\perp}(m,B_i,D,\gamma)=\int\frac{d\Omega}{4\pi}\frac{\sin^2\varphi}{\left[m-\left(B_{\perp}\sin^2\varphi+B_z\cos^2\varphi\right)\right]^2+\sin^2\varphi+\gamma^2\cos^2\varphi+D^2\sin^4\varphi\cos^2 2\theta}, \tag{S69}$$

$$\mathcal{G}_0^{z}(m,B_i,D,\gamma)=\int\frac{d\Omega}{4\pi}\frac{\cos^2\varphi}{\left[m-\left(B_{\perp}\sin^2\varphi+B_z\cos^2\varphi\right)\right]^2+\sin^2\varphi+\gamma^2\cos^2\varphi+D^2\sin^4\varphi\cos^2 2\theta}. \tag{S70}$$

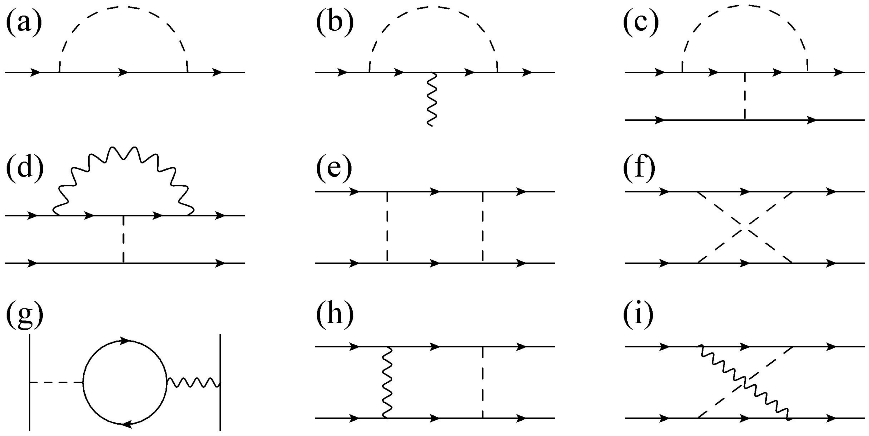


FIG. S2. The Feynman diagrams due to the disorder scattering. The solid, wavy, and dashed lines stand for the fermion, scalar boson, and disorder, respectively.

Here, $m, B_i, D$ are the redefined parameters in Eq. (S34), and we redefine the effective disorder couplings as

$$\frac{\Lambda\Delta_{M,C}}{2\pi^2 v^2\sqrt{\eta}} \to \Delta_{M,C}, \tag{S71}$$

then the disorder-induced self-energy can be rephrased by

$$\Sigma_{\text{dis}}^{(a)}(k_0) = -\left(\Delta_M + \Delta_C\right)\ell\left\{-ik_0\gamma_0\left(\mathcal{G}_0^{\perp} + \mathcal{G}_0^{z}\right) + v\Lambda\left[m\left(\mathcal{G}_0^{\perp} + \mathcal{G}_0^{z}\right) - B_{\perp}\mathcal{G}_0^{\perp} - B_z\mathcal{G}_0^{z}\right]\right\}. \tag{S72}$$

Hereafter, all the parameters are referred to redefined ones. This self-energy gives a correction in the renormalized action by

$$\bar{\psi}\left[G_0^{-1}(k) + \Sigma_{\text{dis}}^{(a)}(k_0)\right]\psi. \tag{S73}$$

Next, we consider Fig. S2(b), which stands for the disorder-induced correction to the vertex of Coulomb interaction and can be written as

$$\begin{aligned}\delta g^{(b)} &= \int\frac{d^3\mathbf{p}}{(2\pi)^3}\left[\Delta_M G_0(0,\mathbf{p})\gamma_0 G_0(0,\mathbf{p}) + \Delta_C\gamma_0 G_0(0,\mathbf{p})\gamma_0 G_0(0,\mathbf{p})\gamma_0\right] \\ &= \left(\Delta_M + \Delta_C\right)\ell\left(\mathcal{G}_0^{\perp} + \mathcal{G}_0^{z}\right)\gamma_0,\end{aligned} \tag{S74}$$

which contributes a correction in the renormalized action according to

$$ig\bar{\psi}\phi\left[\gamma_0 + \delta g^{(b)}\right]\psi. \tag{S75}$$

Fig. S2(c) represents the correction for the disorder vertices caused by the interplay of disorder, it gives rise to

$$\begin{aligned}\delta\Delta_M^{(c)} &= \left(\bar{\psi}_m\psi_m\right)\bar{\psi}_n\left[\int\frac{d^3\mathbf{p}}{(2\pi)^3}\Delta_M G_0(0,\mathbf{p})G_0(0,\mathbf{p}) + \Delta_C\gamma_0 G_0(0,\mathbf{p})G_0(0,\mathbf{p})\gamma_0\right]\psi_n, \\ &= -\left(\Delta_M + \Delta_C\right)\ell\mathcal{G}_1^{z}\left(\bar{\psi}_m\psi_m\right)\left(\bar{\psi}_n\psi_n\right),\end{aligned} \tag{S76}$$

for the random mass, where

$$\mathcal{G}_1^{z}(m, B_i, D, \gamma) = \int\frac{d\Omega}{4\pi}\frac{\left(\sin^2\varphi + \gamma^2\cos^2\varphi\right) + D^2\sin^4\varphi\cos^2 2\theta - \left[m - \left(B_{\perp}\sin^2\varphi + B_z\cos^2\varphi\right)\right]^2}{\left\{\left[m - \left(B_{\perp}\sin^2\varphi + B_z\cos^2\varphi\right)\right]^2 + \sin^2\varphi + \gamma^2\cos^2\varphi + D^2\sin^4\varphi\cos^2 2\theta\right\}^2}. \tag{S77}$$

For the random chemical potential, we obtain

$$\begin{aligned}\delta\Delta_C^{(c)} &= \left(\bar{\psi}_m\gamma_0\psi_m\right)\bar{\psi}_n\left[\int\frac{d^3\mathbf{p}}{(2\pi)^3}\Delta_M G_0(0,\mathbf{p})\gamma_0 G_0(0,\mathbf{p}) + \Delta_C\gamma_0 G_0(0,\mathbf{p})\gamma_0 G_0(0,\mathbf{p})\gamma_0\right]\psi_n \\ &= \left(\Delta_M + \Delta_C\right)\ell\left(\mathcal{G}_0^{\perp} + \mathcal{G}_0^{z}\right)\left(\bar{\psi}_m\gamma_0\psi_m\right)\left(\bar{\psi}_n\gamma_0\psi_n\right).\end{aligned} \tag{S78}$$

This diagram contributes a correction in the renormalized action according to

$$-\left(\frac{2\pi^2 v^2\sqrt{\eta}}{\Lambda}\right)\frac{\Delta_{j=M,C}}{2}\left[\left(\bar{\psi}_m M_j \psi_m\right)\left(\bar{\psi}_n M_j \psi_n\right)+2\delta\Delta_j^{(c)}\right]. \tag{S79}$$

Then, we take into account Fig. S2(d), it stands for the renormalization of the disorder couplings due to the Coulomb interaction, which is given by

$$\delta\Delta_j^{(d)}=\left(\bar{\psi}_m M_j \psi_m\right)\bar{\psi}_n\left[g^2\int\frac{d^3\mathbf{p}}{(2\pi)^3}\int_{-\infty}^{\infty}\frac{dp_0}{2\pi}\gamma_0 G_0(p_0,\mathbf{p})M_j G_0(p_0,\mathbf{p})\gamma_0 D_0(0,\mathbf{p})\right]\psi_n. \tag{S80}$$

For the random chemical potential $M_j=\gamma_0$, we obtain $\delta\Delta_j^{(d)}=0$. For the random mass, $M_j=I$, we have

$$\delta\Delta_j^{(d)}=-\alpha\ell\mathcal{G}_2^z\left(\bar{\psi}_m\psi_m\right)\left(\bar{\psi}_n\psi_n\right), \tag{S81}$$

where,

$$\mathcal{G}_2^z\left(m,B_i,D,\gamma\right)=\int\frac{d\Omega}{4\pi}\frac{\sin^2\varphi+\gamma^2\cos^2\varphi+D^2\sin^4\varphi\cos^2 2\theta}{\left\{\left[m-\left(B_\perp\sin^2\varphi+B_z\cos^2\varphi\right)\right]^2+\sin^2\varphi+\gamma^2\cos^2\varphi+D^2\sin^4\varphi\cos^2 2\theta\right\}^{3/2}}. \tag{S82}$$

As a result, this diagram gives rise to a correction to the renormalized action by

$$-\left(\frac{2\pi^2 v^2\sqrt{\eta}}{\Lambda}\right)\frac{\Delta_M}{2}\left(\bar{\psi}_m\psi_m\right)\left(\bar{\psi}_n\psi_n\right)\left(1+2\alpha\mathcal{G}_2^z\ell\right). \tag{S83}$$

Next, we calculate the disorder vertices corrections coming from the sum of ZS' and BCS type diagrams, exactly Fig. S2(e)+(f), which takes the form

$$\delta\Delta^{(e)+(f)}=\sum_{jl}\Delta_j\Delta_l\int\frac{d^3\mathbf{p}}{(2\pi)^3}\bar{\psi}_m\left[M_j G_0(0,\mathbf{p})M_l\right]\psi_m\bar{\psi}_n\left[M_l G_0(0,\mathbf{p})M_j+M_j G_0(0,-\mathbf{p})M_l\right]\psi_n. \tag{S84}$$

For $j=l=M$ and $C$ we obtain

$$\delta\Delta_{jj}^{(e)+(f)}=\left(\frac{2\pi^2 v^2\sqrt{\eta}}{\Lambda}\right)2\left(\Delta_M^2+\Delta_C^2\right)\ell\left[\mathcal{G}_1^\perp\left(\bar{\psi}_m\psi_m\right)\left(\bar{\psi}_n\psi_n\right)+\mathcal{G}_1^D\left(\bar{\psi}_m i\gamma_5\psi_m\right)\left(\bar{\psi}_n i\gamma_5\psi_n\right)\right], \tag{S85}$$

where

$$\mathcal{G}_1^\perp\left(m,B_i,D,\gamma\right)=\int\frac{d\Omega}{4\pi}\frac{\left[m-\left(B_\perp\sin^2\varphi+B_z\cos^2\varphi\right)\right]^2}{\left\{\left[m-\left(B_\perp\sin^2\varphi+B_z\cos^2\varphi\right)\right]^2+\sin^2\varphi+\gamma^2\cos^2\varphi+D^2\sin^4\varphi\cos^2 2\theta\right\}^2}, \tag{S86}$$

$$\mathcal{G}_1^D\left(m,B_i,D,\gamma\right)=\int\frac{d\Omega}{4\pi}\frac{D^2\sin^4\varphi\cos^2 2\theta}{\left\{\left[m-\left(B_\perp\sin^2\varphi+B_z\cos^2\varphi\right)\right]^2+\sin^2\varphi+\gamma^2\cos^2\varphi+D^2\sin^4\varphi\cos^2 2\theta\right\}^2}. \tag{S87}$$

Note that $\left(\bar{\psi}_m i\gamma_5\psi_m\right)\left(\bar{\psi}_n i\gamma_5\psi_n\right)$ is not present in the original disorder action Eq. (S67). This term represents the dynamically generated disorder described by $H=A_5\left(\bar{\psi}_m i\gamma_5\psi_m\right)$. Considering this term has only the $O(\Delta_j^2)$ contribution. We will neglect this term, and hence we obtain a correction as

$$\delta\Delta_{jj}^{(e)+(f)}=\left(\frac{2\pi^2 v^2\sqrt{\eta}}{\Lambda}\right)2\left(\Delta_M^2+\Delta_C^2\right)\ell\mathcal{G}_1^\perp\left(\bar{\psi}_m\psi_m\right)\left(\bar{\psi}_n\psi_n\right), \tag{S88}$$

which contributes a term to the renormalized action by

$$-\left(\frac{2\pi^2 v^2\sqrt{\eta}}{\Lambda}\right)\frac{\Delta_M}{2}\left(\bar{\psi}_m\psi_m\right)\left(\bar{\psi}_n\psi_n\right)\left[1+2\frac{2\left(\Delta_M^2+\Delta_C^2\right)\mathcal{G}_1^\perp}{\Delta_M}\ell\right]. \tag{S89}$$

For $j\neq l$, we have

$$\delta\Delta_{jl}^{(e)+(f)}=\left(\frac{2\pi^2 v^2\sqrt{\eta}}{\Lambda}\right)2\Delta_M\Delta_C\ell\left[\mathcal{G}_1^\perp\left(\bar{\psi}_m\gamma_0\psi_m\right)\left(\bar{\psi}_n\gamma_0\psi_n\right)+\mathcal{G}_1^j\left(\bar{\psi}_m\gamma_0\gamma_j\psi_m\right)\left(\bar{\psi}_n\gamma_0\gamma_j\psi_n\right)\right], \tag{S90}$$

where

$$\mathcal{G}_1^{j=(1,2,3)}(m, B_i, D, \gamma) = \int \frac{d\Omega}{4\pi} \frac{\left(1/2\sin^2\varphi, 1/2\sin^2\varphi, \gamma^2\cos^2\varphi\right)}{\left\{\left[m - \left(B_\perp \sin^2\varphi + B_z \cos^2\varphi\right)\right]^2 + \sin^2\varphi + \gamma^2\cos^2\varphi + D^2\sin^4\varphi\cos^2 2\theta\right\}^2}. \quad \text{(S91)}$$

Similar to the previous results, we think $\left(\bar{\psi}_m\gamma_0\gamma_i\psi_m\right)\left(\bar{\psi}_n\gamma_0\gamma_i\psi_n\right)$ is a higher-order correction and can be ignored directly, as a result,

$$\delta\Delta_{jl}^{(e)+(f)} = \left(\frac{2\pi^2 v^2\sqrt{\eta}}{\Lambda}\right) 2\Delta_M\Delta_C\ell\mathcal{G}_1^\perp \left(\bar{\psi}_m\gamma_0\psi_m\right)\left(\bar{\psi}_n\gamma_0\psi_n\right), \quad \text{(S92)}$$

which contributes a term to the renormalized action by

$$-\left(\frac{2\pi^2 v^2\sqrt{\eta}}{\Lambda}\right)\frac{\Delta_C}{2}\left(\bar{\psi}_m\gamma_0\psi_m\right)\left(\bar{\psi}_n\gamma_0\psi_n\right)\left(1 + 4\Delta_M\mathcal{G}_1^\perp\ell\right). \quad \text{(S93)}$$

The defined $\mathcal{G}_0^\perp, \mathcal{G}_0^z, \mathcal{G}_1^\perp, \mathcal{G}_1^z$ are not fully independent. Instead, they satisfy

$$\mathcal{G}_0^\perp + \mathcal{G}_0^z = 2\mathcal{G}_1^\perp + \mathcal{G}_1^z. \quad \text{(S94)}$$

We now calculate Fig. S2(g), which gives rise to a correction to the disorder vertex and takes the form

$$\delta\Delta_j^{(g)} = \Delta_j g^2\left[\left(\bar{\psi}_m M_j\psi_m\right)\int\frac{d^3\mathbf{q}}{(2\pi)^3}\int_{-\infty}^{\infty}\frac{dq_0}{2\pi} - \mathrm{Tr}\left[M_j G_0\left(q_0,\mathbf{q}\right)\gamma_0 G_0\left(q_0,\mathbf{k}+\mathbf{q}\right)\right]D_0(0,\mathbf{k})\left(\bar{\psi}_n\gamma_0\psi_n\right)\right]. \quad \text{(S95)}$$

Only $M_j = \gamma_0$ does not vanish in the trace, and the corresponding result is same as Eq. (S57),

$$\delta\Delta_C^{(g)} = \Delta_C\alpha\ell\left(\bar{\psi}_m\gamma_0\psi_m\right)\left(\bar{\psi}_n\gamma_0\psi_n\right)\left[\frac{\mathcal{F}_2^\perp(m, B_i, D, \gamma)\,k_\perp^2 + \mathcal{F}_2^z(m, B_i, D, \gamma)\,\eta k_z^2}{k_\perp^2 + \eta k_z^2}\right]. \quad \text{(S96)}$$

Due to the existence of the anisotropy, this correction is highly dependent on the external momentum which is extremely smaller than the integral momentum. To get a momentum-independent correction, we temporarily take $\mathcal{F}_2^\perp(m, B_i, D, \gamma) \approx \mathcal{F}_2^z(m, B_i, D, \gamma)$ and we show that this approximation is well established in the low-energy limit. After taking this approximation, we obtain

$$\delta\Delta_C^{(g)} = \Delta_C\alpha\mathcal{F}_2^\perp(m, B_i, D, \gamma)\,\ell\left(\bar{\psi}_m\gamma_0\psi_m\right)\left(\bar{\psi}_n\gamma_0\psi_n\right), \quad \text{(S97)}$$

which generates a term in the renormalized action as

$$-\left(\frac{2\pi^2 v^2\sqrt{\eta}}{\Lambda}\right)\frac{\Delta_C}{2}\left(\bar{\psi}_m\gamma_0\psi_m\right)\left(\bar{\psi}_n\gamma_0\psi_n\right)\left(1 - 2\alpha\mathcal{F}_2^\perp\ell\right). \quad \text{(S98)}$$

At last, we consider the corrections due to Fig. S2(h)+(i), which are similar to Fig. S2(e)+(f), and reads

$$\delta\Delta^{(h)+(i)} = \Delta_j g^2\int\frac{d^3\mathbf{p}}{(2\pi)^3}\bar{\psi}_m\left[\gamma_0 G_0(0,\mathbf{p})M_j\right]\psi_m\bar{\psi}_n\left[M_j G_0(0,\mathbf{p})\gamma_0 + \gamma_0 G_0(0,-\mathbf{p})M_j\right]\psi_n D_0(\mathbf{p}). \quad \text{(S99)}$$

The momentum integral is highly suppressed due to term of $D_0(\mathbf{p}) = \frac{1}{p_\perp^2 + \eta p_z^2}$. As a result, this correction is proportional to $\alpha\ell/(v\Lambda)$, which is irrelevant and can be ignored directly. This suppression reflects that Fig. S2(e)+(f) is not UV divergent if we consider the renormalization beyond the Wilson's approach [11].

### C. Renormalization group equations

After collecting all the one-loop corrections, we first perform rescaling of the space-time coordinates as $(\mathbf{r}_x, \mathbf{r}_y) \to (\mathbf{r}_x, \mathbf{r}_y)e^\ell$, $\tau \to \tau e^{\kappa\ell}$, $\mathbf{r}_z \to \mathbf{r}_z e^{\kappa_1\ell}$, and then introduce the renormalization constants according to $\psi \to Z_\psi^{-1/2}\psi, \phi \to$

$Z_{\phi}^{-1/2}\phi, g \to Z_{g^2}^{-1/2}g$, $v \to Z_{v_i}^{-1}v_i, \eta \to Z_{\eta}^{-1}\eta, \alpha \to Z_{g^2}^{-1}Z_v Z_{\eta}^{1/2}\alpha = Z_{\alpha}^{-1}\alpha, m \to Z_m^{-1}m$, $B_i \to Z_{B_i}^{-1}B_i$, and $D \to Z_D^{-1}D$. The action rephrased by the renormalized parameters and rescaled coordinates takes the form

$$\begin{aligned}\mathcal{S}' = &\int d\tau d^3\mathbf{r} e^{(\kappa+\kappa_1+2)\ell}\Bigg\{\frac{\bar{\psi}}{Z_\psi}\Bigg[e^{-\kappa\ell}\left[1+(\Delta_M+\Delta_C)\ell\left(\mathcal{G}_0^\perp+\mathcal{G}_0^z\right)\right]\gamma_0\partial_0+\frac{ig\gamma_0\phi}{\sqrt{Z_{g^2}Z_\phi}}\left[1+(\Delta_M+\Delta_C)\left(\mathcal{G}_0^\perp+\mathcal{G}_0^z\right)\ell\right]\\
&+\frac{ve^{-\ell}}{Z_v}\left(1+\alpha\ell\mathcal{F}_0^\perp\right)(\gamma_x\partial_x+\gamma_y\partial_y)+\frac{v_z e^{-\kappa_1\ell}}{Z_{v_z}}\left(1+2\alpha\ell\mathcal{F}_0^z\right)\gamma_z\partial_z+\frac{mv\Lambda}{Z_m Z_v}\Bigg[1+\alpha\ell\Bigg(\mathcal{F}_0^\perp+\mathcal{F}_0^z-\frac{B_\perp\mathcal{F}_0^\perp+B_z\mathcal{F}_0^z}{m}\Bigg)\\
&-(\Delta_M+\Delta_C)\ell\left(\mathcal{G}_0^\perp+\mathcal{G}_0^z-\frac{B_\perp\mathcal{G}_0^\perp+B_z\mathcal{G}_0^z}{m}\right)\Bigg]+\frac{B_\perp v\Lambda^{-1}}{Z_{B_\perp}Z_v}\left[1+\alpha\ell\left(\mathcal{F}_1^\perp+\frac{B_z\mathcal{F}_1^z-m\left(\mathcal{F}_1^\perp+\mathcal{F}_1^z\right)}{B_\perp}\right)\right]\\
&\times e^{-2\ell}\left(\partial_x^2+\partial_y^2\right)+\frac{B_z v\Lambda^{-1}\eta}{Z_{B_z}Z_v Z_\eta}\Big\{1+\alpha\ell\Big[\left(\mathcal{F}_0^z-2\mathcal{F}_1^z\right)+B_\perp\left(\mathcal{F}_0^\perp-2\mathcal{F}_1^\perp\right)/B_z-m\big[\mathcal{F}_0^\perp+\mathcal{F}_0^z\\
&-2\left(\mathcal{F}_1^\perp+\mathcal{F}_1^z\right)\big]/B_z\Big]\Big\}e^{-2\kappa_1\ell}\partial_z^2-\frac{iDv\Lambda^{-1}}{Z_v Z_D}\gamma_5\left(1+\alpha\mathcal{F}_1^D\ell\right)e^{-2\ell}\left(\partial_x^2-\partial_y^2\right)\Bigg]\psi\\
&+\frac{1}{2}\left[\frac{e^{-2\ell}}{Z_\phi}\left(1+\alpha\mathcal{F}_2^\perp\ell\right)\left[(\partial_x\phi)^2+(\partial_y\phi)^2\right]+\frac{e^{-2\kappa_1\ell}}{Z_\phi Z_\eta}\left(1+\alpha\mathcal{F}_2^z\ell\right)\eta(\partial_z\phi)^2\right]\Bigg\}.\end{aligned}\tag{S100}$$

The renormalized disorder action after rescaling becomes

$$\begin{aligned}\mathcal{S}_{\text{dis}}' = &-\frac{1}{2}\int d^3\mathbf{r}d\tau d\tau' e^{(2\kappa+\kappa_1+2)\ell}\left(\frac{2\pi^2v^2\sqrt{\eta}}{\Lambda Z_v^2\sqrt{Z_\eta}}\right)\Bigg\{\frac{\Delta_M}{Z_{\Delta_M}Z_\psi^2}\left(\bar{\psi}_m\psi_m\right)_r\left(\bar{\psi}_n\psi_n\right)_{r'}\Big[1-2\left(\Delta_M+\Delta_C\right)\ell\mathcal{G}_1^z+2\alpha\ell\mathcal{G}_2^z\\
&+4\left(\Delta_M^2+\Delta_C^2\right)\ell\mathcal{G}_1^\perp/\Delta_M\Big]+\frac{\Delta_C}{Z_{\Delta_C}Z_\psi^2}\left(\bar{\psi}_m\gamma_0\psi_m\right)_r\left(\bar{\psi}_n\gamma_0\psi_n\right)_{r'}\Big[1+2\left(\Delta_C+\Delta_M\right)\ell\left(\mathcal{G}_0^\perp+\mathcal{G}_0^z\right)\\
&+4\Delta_M\ell\mathcal{G}_1^\perp-2\alpha\ell\mathcal{F}_2^\perp\Big]\Bigg\}.\end{aligned}\tag{S101}$$

By requiring that $\mathcal{S}'$ takes the same form as $\mathcal{S}$ (Eq. (S24)) but with rescaled space, time, fields, and parameters, we could obtain the renormalized constants $Z_\psi, Z_\phi$ for fields and $Z_{g^2}, Z_{v_i}, Z_\eta, Z_m, Z_{B_i}, Z_D, Z_\alpha$ for the parameters. Similarly, by requiring that $\mathcal{S}_{\text{dis}}'$ takes the same form as $S_{\text{dis}}$ (Eq. (S67)), we obtain the renormalized constants $Z_{\Delta_M}, Z_{\Delta_C}$ for the disorder coupling parameters. Specifically,

$$\begin{aligned}Z_\psi &= e^{(\kappa_1+2)\ell}\left[1+(\Delta_M+\Delta_C)\ell\left(\mathcal{G}_0^\perp+\mathcal{G}_0^z\right)\right],\\
Z_\phi &= e^{(\kappa+\kappa_1)\ell}\left(1+\alpha\mathcal{F}_2^\perp\ell\right),\\
Z_{g^2} &= e^{(\kappa-\kappa_1)\ell}\left(1-\alpha\mathcal{F}_2^\perp\ell\right),\\
Z_v &= e^{(\kappa-1)\ell}\left[1+\mathcal{F}_0^\perp\alpha\ell-(\Delta_M+\Delta_C)\ell\left(\mathcal{G}_0^\perp+\mathcal{G}_0^z\right)\right],\\
Z_{v_z} &= e^{(\kappa-\kappa_1)\ell}\left[1+2\mathcal{F}_0^z\alpha\ell-(\Delta_M+\Delta_C)\ell\left(\mathcal{G}_0^\perp+\mathcal{G}_0^z\right)\right],\\
Z_m &= e^{\ell}\left[1+\alpha\ell\left(\mathcal{F}_0^z-\frac{B_\perp\mathcal{F}_0^\perp+B_z\mathcal{F}_0^z}{m}\right)-(\Delta_M+\Delta_C)\ell\left(\mathcal{G}_0^\perp+\mathcal{G}_0^z-\frac{B_\perp\mathcal{G}_0^\perp+B_z\mathcal{G}_0^z}{m}\right)\right],\\
Z_{B_\perp} &= e^{-\ell}\left[1+\alpha\ell\left(\mathcal{F}_1^\perp-\mathcal{F}_0^\perp+\frac{B_z\mathcal{F}_1^z-m\left(\mathcal{F}_1^\perp+\mathcal{F}_1^z\right)}{B_\perp}\right)\right],\\
Z_{B_z} &= e^{-\ell}\Big\{1+\alpha\ell\Big[\left(\mathcal{F}_2^\perp-\mathcal{F}_2^z-\mathcal{F}_0^\perp+\mathcal{F}_0^z-2\mathcal{F}_1^z\right)+B_\perp\left(\mathcal{F}_0^\perp-2\mathcal{F}_1^\perp\right)/B_z-m\big[\mathcal{F}_0^\perp+\mathcal{F}_0^z-2\left(\mathcal{F}_1^\perp+\mathcal{F}_1^z\right)\big]/B_z\Big]\Big\},\\
Z_D &= e^{-\ell}\left[1+\alpha\ell\left(\mathcal{F}_1^D-\mathcal{F}_0^\perp\right)\right],\\
Z_\eta &= e^{2(1-\kappa_1)\ell}\left[1+\alpha\ell\left(\mathcal{F}_2^z-\mathcal{F}_2^\perp\right)\right],\\
Z_{\Delta_M} &= e^{-\ell}\left\{1-2\left(\Delta_M+\Delta_C\right)\ell\mathcal{G}_1^z+\alpha\ell\left[2\left(\mathcal{G}_2^z-\mathcal{F}_0^\perp\right)+\left(\mathcal{F}_2^\perp-\mathcal{F}_2^z\right)/2\right]+4\left(\Delta_M^2+\Delta_C^2\right)\ell\mathcal{G}_1^\perp/\Delta_M\right\},\\
Z_{\Delta_C} &= e^{-\ell}\left\{1+2\left(\Delta_C+\Delta_M\right)\ell\left(\mathcal{G}_0^\perp+\mathcal{G}_0^z\right)+4\Delta_M\ell\mathcal{G}_1^\perp-\alpha\ell\left[2\mathcal{F}_0^\perp+\left(3\mathcal{F}_2^\perp+\mathcal{F}_2^z\right)/2\right]\right\},\\
Z_\alpha &= \frac{Z_{g^2}}{Z_v\sqrt{Z_\eta}} = 1-\mathcal{F}_0^\perp\alpha\ell+(\Delta_M+\Delta_C)\ell\left(\mathcal{G}_0^\perp+\mathcal{G}_0^z\right)-\alpha\ell\left(\mathcal{F}_2^z+\mathcal{F}_2^\perp\right)/2,\\
Z_\gamma &= \frac{Z_{v_z}}{Z_v\sqrt{Z_\eta}} = 1+\left(2\mathcal{F}_0^z\alpha-\mathcal{F}_0^\perp\right)\ell-\alpha\ell\left(\mathcal{F}_2^z-\mathcal{F}_2^\perp\right)/2.\end{aligned}\tag{S102}$$

The renormalization group equations for the parameters are obtained according to

$$\frac{d\ln X}{d\ell} = \left.\frac{dZ_X}{d\ell}\right|_{\ell\to 0}, \text{ (X denotes the parameters but not fields)} \tag{S103}$$

which are given by

$$\begin{aligned}
\frac{dv}{d\ell} &= \left[\kappa - 1 + \mathcal{F}_0^{\perp}\alpha - (\Delta_M + \Delta_C)\left(\mathcal{G}_0^{\perp} + \mathcal{G}_0^{z}\right)\right] v, \\
\frac{dv_z}{d\ell} &= \left[\kappa - \kappa_1 + 2\mathcal{F}_0^{z}\alpha - (\Delta_M + \Delta_C)\left(\mathcal{G}_0^{\perp} + \mathcal{G}_0^{z}\right)\right] v_z, \\
\frac{dm}{d\ell} &= m + \alpha\left[m\mathcal{F}_0^{z} - \left(B_\perp\mathcal{F}_0^{\perp} + B_z\mathcal{F}_0^{z}\right)\right] - (\Delta_M + \Delta_C)\left[m\left(\mathcal{G}_0^{\perp} + \mathcal{G}_0^{z}\right) - \left(B_\perp\mathcal{G}_0^{\perp} + B_z\mathcal{G}_0^{z}\right)\right], \\
\frac{dB_\perp}{d\ell} &= -B_\perp + \alpha\left[B_\perp\left(\mathcal{F}_1^{\perp} - \mathcal{F}_0^{\perp}\right) + \left(B_z\mathcal{F}_1^{z} - m\mathcal{F}_1^{\perp} - m\mathcal{F}_1^{z}\right)\right], \\
\frac{dB_z}{d\ell} &= -B_z + \alpha\Big[B_z\left(\mathcal{F}_2^{\perp} - \mathcal{F}_2^{z} - 2\mathcal{F}_1^{z}\right) + B_\perp\left(\mathcal{F}_0^{\perp} - 2\mathcal{F}_1^{\perp}\right) - m\left(\mathcal{F}_0^{\perp} + \mathcal{F}_0^{z} - 2\mathcal{F}_1^{\perp} - 2\mathcal{F}_1^{z}\right)\Big], \\
\frac{dD}{d\ell} &= \left[-1 + \alpha\left(\mathcal{F}_1^{D} - \mathcal{F}_0^{\perp}\right)\right] D, \\
\frac{d\Delta_M}{d\ell} &= -\Delta_M - 2\Delta_M^2\left(\mathcal{G}_1^{z} - 2\mathcal{G}_1^{\perp}\right) - 2\Delta_C\Delta_M\mathcal{G}_1^{z} + 4\Delta_C^2\mathcal{G}_1^{\perp} + \alpha\Delta_M\left[2\left(\mathcal{G}_2^{z} - \mathcal{F}_0^{\perp}\right) + \frac{\mathcal{F}_2^{\perp} - \mathcal{F}_2^{z}}{2}\right], \\
\frac{d\Delta_C}{d\ell} &= -\Delta_C + 2\Delta_C\left(\Delta_C + \Delta_M\right)\left(\mathcal{G}_0^{\perp} + \mathcal{G}_0^{z}\right) + 4\Delta_M\Delta_C\mathcal{G}_1^{\perp} - \alpha\Delta_C\left[2\mathcal{F}_0^{\perp} + \left(3\mathcal{F}_2^{\perp} + \mathcal{F}_2^{z}\right)/2\right], \\
\frac{d\alpha}{d\ell} &= -\alpha^2\left(\mathcal{F}_0^{\perp} + \frac{\mathcal{F}_2^{z} + \mathcal{F}_2^{\perp}}{2}\right) + \alpha\left(\Delta_M + \Delta_C\right)\left(\mathcal{G}_0^{\perp} + \mathcal{G}_0^{z}\right), \\
\frac{d\gamma^2}{d\ell} &= \gamma^2\alpha\left[2\left(2\mathcal{F}_0^{z} - \mathcal{F}_0^{\perp}\right) - \mathcal{F}_2^{z} + \mathcal{F}_2^{\perp}\right].
\end{aligned} \tag{S104}$$

By requiring that $v$ and $v_z$ are scale-invariant, the dynamical exponent and anomalous $z$-dimension are obtained as

$$\kappa = 1 - \alpha\mathcal{F}_0^{\perp} + (\Delta_M + \Delta_C)\left(\mathcal{G}_0^{\perp} + \mathcal{G}_0^{z}\right), \tag{S105}$$

$$\kappa_1 = 1 + \left(2\mathcal{F}_0^{z} - \mathcal{F}_0^{\perp}\right)\alpha. \tag{S106}$$

Taking $\Delta_M = \Delta_C = 0$ and considering Eq. (S43), Eq. (S94), the renormalization-group equations are simplified to be Eq. (5)-(11) in the main text.

## SV. INFLUENCE OF COULOMB INTERACTION STRENGTH

We display our results by varying the initial values of $D$ in the main text. To show the influence of the Coulomb interaction strength, we plot more results by varying the initial values of $\alpha$ and keeping other parameters fixed.

Figures S3(a) and (b) show that $D$ flows to zero while $m$ does not change sign. Figure S3(c) shows that $\alpha$ flows to a constant but nonzero. Figure S3(d) shows that $\kappa$ flows to 1. Therefore, the phase transition from second-order topological insulator to topological insulator is highly independent on the strength of the effective Coulomb interaction, at least for $\alpha > 10^{-3}$.

Figure S3(a) shows that the sign change of $m$ happens only when $\alpha$ is large enough. The phase transition from second-order topological insulator to normal insulator is highly dependent on the strength of the effective Coulomb interaction. This phase transition exists only when the effective Coulomb interaction is larger than a critical value, and the value of the strength is determined by the values of the band parameters.

## SVI. INFLUENCE OF DISORDER

### A. Random mass

To consider the influence of random mass to our conclusions, we take $\Delta_C = 0$, the RG equations for $B_i$, $D$ and $\gamma^2$ in the main text are unchanged, while the RG equations for $m$, $\alpha$ and $\Delta_M$ become

$$\frac{dm}{d\ell} = m + \alpha\left[m\mathcal{F}_0^{z} - \left(B_\perp\mathcal{F}_0^{\perp} + B_z\mathcal{F}_0^{z}\right)\right] - \Delta_M\left[m\left(\mathcal{G}_0^{\perp} + \mathcal{G}_0^{z}\right) - \left(B_\perp\mathcal{G}_0^{\perp} + B_z\mathcal{G}_0^{z}\right)\right],$$

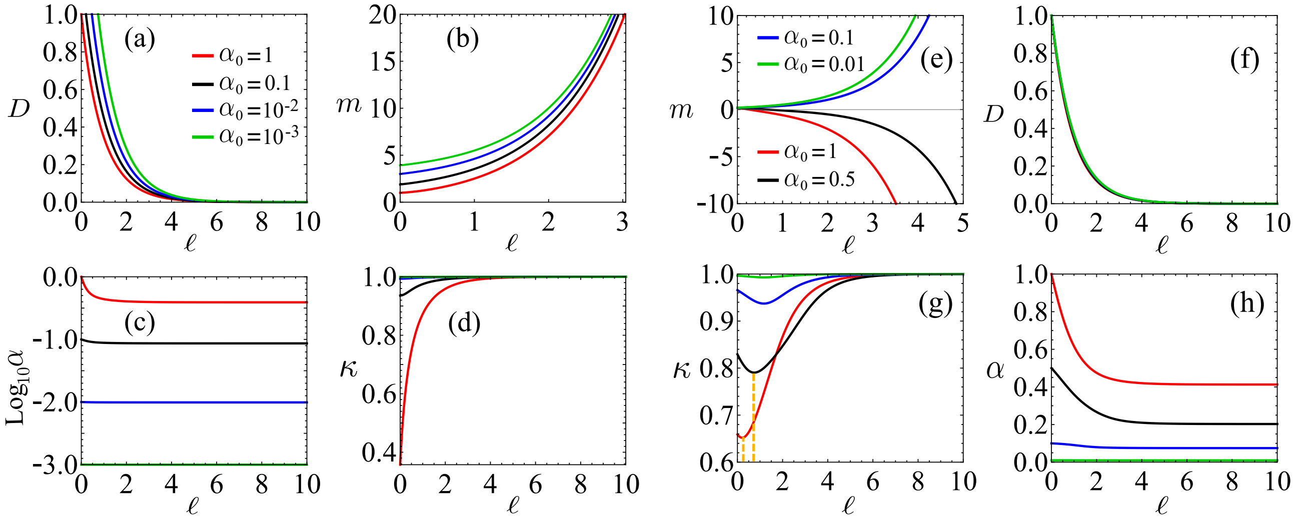


FIG. S3. [(a)-(c)] Numerical solutions to the renormalized $m$, $D$, and $\alpha$ as functions of the running scale parameter $\ell$. (d) The scale dependence of $\kappa$. For [(a)-(d)], the solutions are obtained by varying the initial value $\alpha$ and fixing the initial values of other parameters as $m_0 = B_\perp^0 = B_z^0 = D_0 = 1$, $\gamma_0 = 0.5$, which corresponds to a second-order topological insulator. (a)–(d) share the same legends. [(e), (f), (h)] Numerical solutions to the renormalized $m$, $D$, and $\alpha$ as functions of the running scale parameter $\ell$. (g) The scale dependence of $\kappa$. For (e)-(h), the solutions are obtained by varying the initial value $D$ and fixing the initial values of other parameters as $m_0 = 0.2, B_\perp^0 = 2D_0 = 2, B_z^0 = 1.3$, $\gamma_0 = 0.25$, which is a second-order topological insulator. (e)–(h) share the same legends. The orange dashed lines in (c) label the values of $\ell$ at which the topological phase transitions happen, and the crossing points of the orange dashed lines with the red and black lines indicate the corresponding values of $\kappa$, which are $0.66, 0.79$, respectively.

$$\frac{d\Delta_M}{d\ell} = -\Delta_M - 2\Delta_M^2\left(\mathcal{G}_1^z - 2\mathcal{G}_1^\perp\right) + \alpha\Delta_M\left[2\left(\mathcal{G}_2^z - \mathcal{F}_0^\perp\right) + \frac{\mathcal{F}_2^\perp - \mathcal{F}_2^z}{2}\right],$$
$$\frac{d\alpha}{d\ell} = -\alpha^2\left(\mathcal{F}_0^\perp + \frac{\mathcal{F}_2^z + \mathcal{F}_2^\perp}{2}\right) + \alpha\Delta_M\left(\mathcal{G}_0^\perp + \mathcal{G}_0^z\right). \tag{S107}$$

Therefore, $\Delta_M$ plays a similar role as the Coulomb interaction, and hence the random mass cannot stop the unrestricted increase or decrease of $m$. In the low-energy limit, $\mathcal{F}_{0,1}^{\perp,z} \sim 1/|m| \sim 0$, $\mathcal{G}_{0,1}^{\perp,z} \sim 1/m^2 \sim 0$, $\mathcal{F}_2^{\perp,z}, \mathcal{G}_2^z \sim 1/|m|^3 \sim 0$, and hence $\Delta_M^* = 0$ is the only stable fixed point. The random mass is an irrelevant perturbation and nearly ignorable. The main conclusions in the main text do not change when the random mass disorder exist. To explicitly show this, we re-plot Fig. 2 in Fig. S4 and Fig. 3 in Fig. S5 by numerically solve the coupled RG equations when the random mass exists. By comparing Fig. S4 with Fig. 2, we see that the random mass does not influence our conclusions in nature except that it slightly changes the running behavior of $m$ and $\alpha$. This is mainly due to the irrelevance of $\Delta_M$, which is shown in Fig. S4(e). By comparing Fig. S5 with Fig. 3, we see that the transition between HOTIs and normal insulators still could happen when the Coulomb interaction coexist with the random mass disorder. This is mainly due to the irrelevance of $\Delta_M$, which is shown in Fig. S5(e). However, due to the renormalization of $m$ by the random mass, the condition for the phase transition is different from the clean system. For example, the blue line in Fig. S5 represents a phase transition to topological insulator, while it corresponds to a phase transition to normal insulator in Fig. 3 of the main text. Therefore, the presence of the random mass does not influence the existence of these two kinds of phase transition but just slightly change their boundaries in the multi-parameter plain.

### B. Random chemical potential

By taking $\Delta_M = 0$, the RG equations for $m$, $\alpha$, and $\Delta_C$ become

$$\frac{dm}{d\ell} = m + \alpha\left[m\mathcal{F}_0^z - \left(B_\perp\mathcal{F}_0^\perp + B_z\mathcal{F}_0^z\right)\right] - \Delta_C\left[m\left(\mathcal{G}_0^\perp + \mathcal{G}_0^z\right) - \left(B_\perp\mathcal{G}_0^\perp + B_z\mathcal{G}_0^z\right)\right],$$
$$\frac{d\Delta_C}{d\ell} = -\Delta_C + 2\Delta_C^2\left(\mathcal{G}_0^\perp + \mathcal{G}_0^z\right) - \alpha\Delta_C\left[2\mathcal{F}_0^\perp + \left(3\mathcal{F}_2^\perp + \mathcal{F}_2^z\right)/2\right],$$
$$\frac{d\alpha}{d\ell} = -\alpha^2\left(\mathcal{F}_0^\perp + \frac{\mathcal{F}_2^z + \mathcal{F}_2^\perp}{2}\right) + \alpha\Delta_C\left(\mathcal{G}_0^\perp + \mathcal{G}_0^z\right). \tag{S108}$$

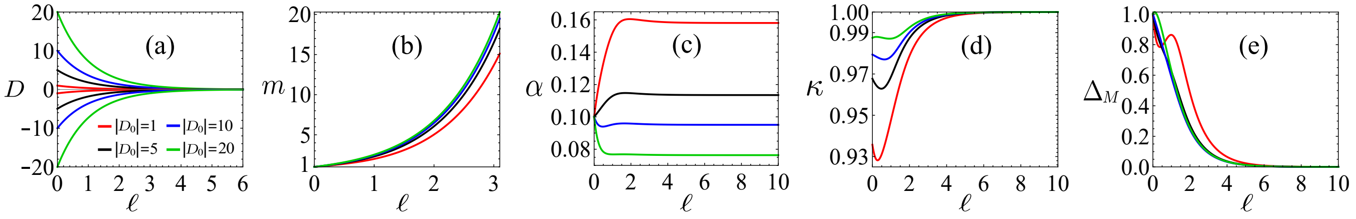


FIG. S4. [(a)-(e)] Numerical solutions to the renormalized $D$, $m$, $\alpha$, $\kappa$ and $\Delta_M$ as functions of the running scale parameter $\ell$. The solutions are obtained by fixing the values at $\ell = 0$ as $m_0 = B_\perp^0 = \Delta_M^0 = 1$, $B_z^0 = 0.5$, $\alpha_0 = 0.1 = \gamma_0^2 = 0.1$ while varying $D_0$. (a)–(e) share the same legends. Except $\Delta_M^0 = 1$, the initial values of other parameters are the same as those of Fig. 2 in the main text.

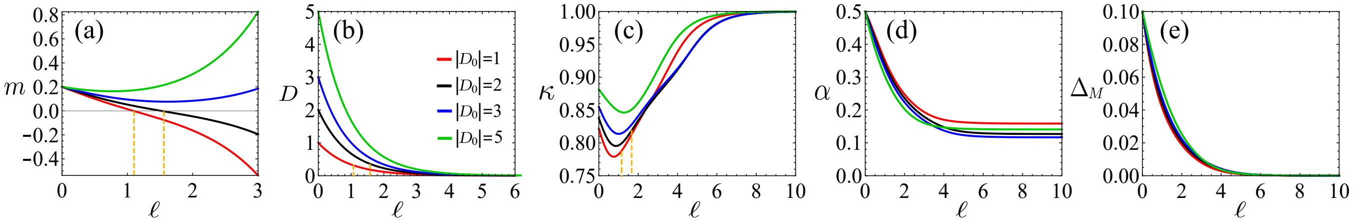


FIG. S5. [(a)-(e)] Numerical solutions to the renormalized $m$, $D$, $\kappa$, $\alpha$ and $\Delta_M$ as functions of the running scale parameter $\ell$. The solutions are obtained by fixing the values at $\ell = 0$ as $m_0 = B_\perp^0 = \Delta_M^0 = 1$, $m_0 = 0.2$, $B_\perp^0 = 2B_z^0 = 2$, $\alpha_0 = 0.5$, and $\Delta_M = \gamma_0^2 = 0.1$ while varying $D_0$. (a)–(e) share the same legends. Except $\Delta_M^0 = 0.1$, the initial values of other parameters are the same as those in Fig. 3 of the main text.

Therefore, the RG equation for $\Delta_C$ can be rewritten as $d\Delta_C/d\ell = -a\Delta_C^2 + b\Delta_C$ where $a$ and $b$ are two positive parameters. Once we fix our model parameters as constants, we could schematically plot $d\Delta_C/d\ell = -a\Delta_C^2 + b\Delta_C$, as shown in Fig. S6. According to Fig. S6, $d\Delta_C/d\ell$ has a root as $\Delta_C^c = b/a$, and once $\Delta_C^0 > \Delta_C^c$, $d\Delta_C/d\ell$ is positive, as a result, $\Delta_C$ will increase unboundedly with increasing $\ell$, which signifies a phase transition to a strong-disorder dominated compressible diffusive metal. The blue and green lines in the Fig. 4(b) of the main text display this case. If $\Delta_C^0 < \Delta_C^c$, $d\Delta_C/d\ell$ is negative, $\Delta_C$ will flow to the Gaussian fixed point, which means that the random chemical potential is also irrelevant. The red and black lines in Fig. 4(b) of the main text display this case. For the irrelevant random chemical potential, its influence to our conclusions will be the same as the random mass, which has been analyzed previously. Here, we have taken a constant value of $\Delta_C^c$ to understand the flow behavior of $\Delta(\ell)$. In real cases, the specific value of $\Delta_C^c$ is also changed with varying $\ell$. Once $\Delta_C^0 > (\Delta_C^c(\ell))_{\max}$ the compressible diffusive metal happens. The understanding by using a fixed $\Delta_C^c$ is still established.

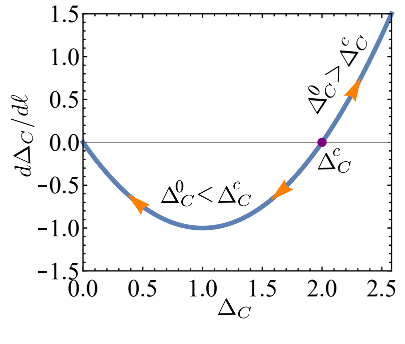


FIG. S6. A sketch for the dependence of $\frac{d\Delta_C}{d\ell}$ on $\Delta_C$. Here $\Delta_C^c$ accounts for a critical value of $\Delta_C$, and $\Delta_C^c$ means its initial value. The curve is plotted by using a function $f(x) = x^2 - 2x$.

[1] F. Schindler, A. M. Cook, M. G. Vergniory, Z. Wang, S. S. P. Parkin, B. A. Bernevig, and T. Neupert, Sci. Adv. **4**, 6 (2018).
[2] L. Fu, C. L. Kane, and E. J. Mele, Phys. Rev. Lett. **98**, 106803 (2007).
[3] L. Fu and C. L. Kane, Phys. Rev. B **76**, 045302 (2007).
[4] A. W. W. Ludwig, M. P. A. Fisher, R. Shankar, and G. Grinstein, Phys. Rev. B **50**, 7526 (1994).
[5] A. A. Nersesyan, A. M. Tsvelik, and F. Wenger, Nucl. Phys. B **438**, 561 (1995).
[6] A. Altland, B. Simons, and M. Zirnbauer, Phys. Rep. **359**, 283 (2002).
[7] T. Stauber, F. Guinea, and M. A. H. Vozmediano, Phys. Rev. B **71**, 041406 (2005).
[8] P. A. Lee and T. V. Ramakrishnan, Rev. Mod. Phys. **57**, 287 (1985).
[9] A. Altland and B. D. Simons, *Condensed matter field theory* (Cambridge University Press, 2010).
[10] P. Coleman, *Introduction to Many-Body Physics* (Cambridge University Press, Cambridge, 2015).
[11] M. E. Peskin and D. V. Schroeder, *An Introduction to Quantum Field Theory* (CRC Press, 2019).
